# Supplementary material for: Observation of a pronounced Hebel-Slichter peak in the spin-lattice relaxation rate and implications for gap and pairing symmetry in LaNiGa$_2$
Source: arXiv:2510.23800 source file (2025-10-27)
Supplement: Supplementary file 1 [file supplemental.pdf]

# Supplemental Materials: Observation of a pronounced Hebel-Slichter peak in the spin-lattice relaxation rate and implications for gap and pairing symmetry in $LaNiGa_2$

P. Sherpa,[1] Rahul Hingorani,[1] Anirudha Menon,[1] I. Vinograd,[1] C. Chaffey,[1] A. P. Dioguardi,[2] R. Yamamoto,[2] M. Hirata,[2] F. Ronning,[2] J. R. Badger,[3] P. Klavins,[1] Rajiv Singh,[1] V. Taufour,[1] and N. J. Curro[1]

[1]*Department of Physics and Astronomy, University of California, Davis, California 95616, USA*

[2]*Los Alamos National Laboratory, Los Alamos, New Mexico 87545, USA*

[3]*Department of Chemistry, University of California, Davis, California 95616, USA*

(Dated: October 27, 2025)

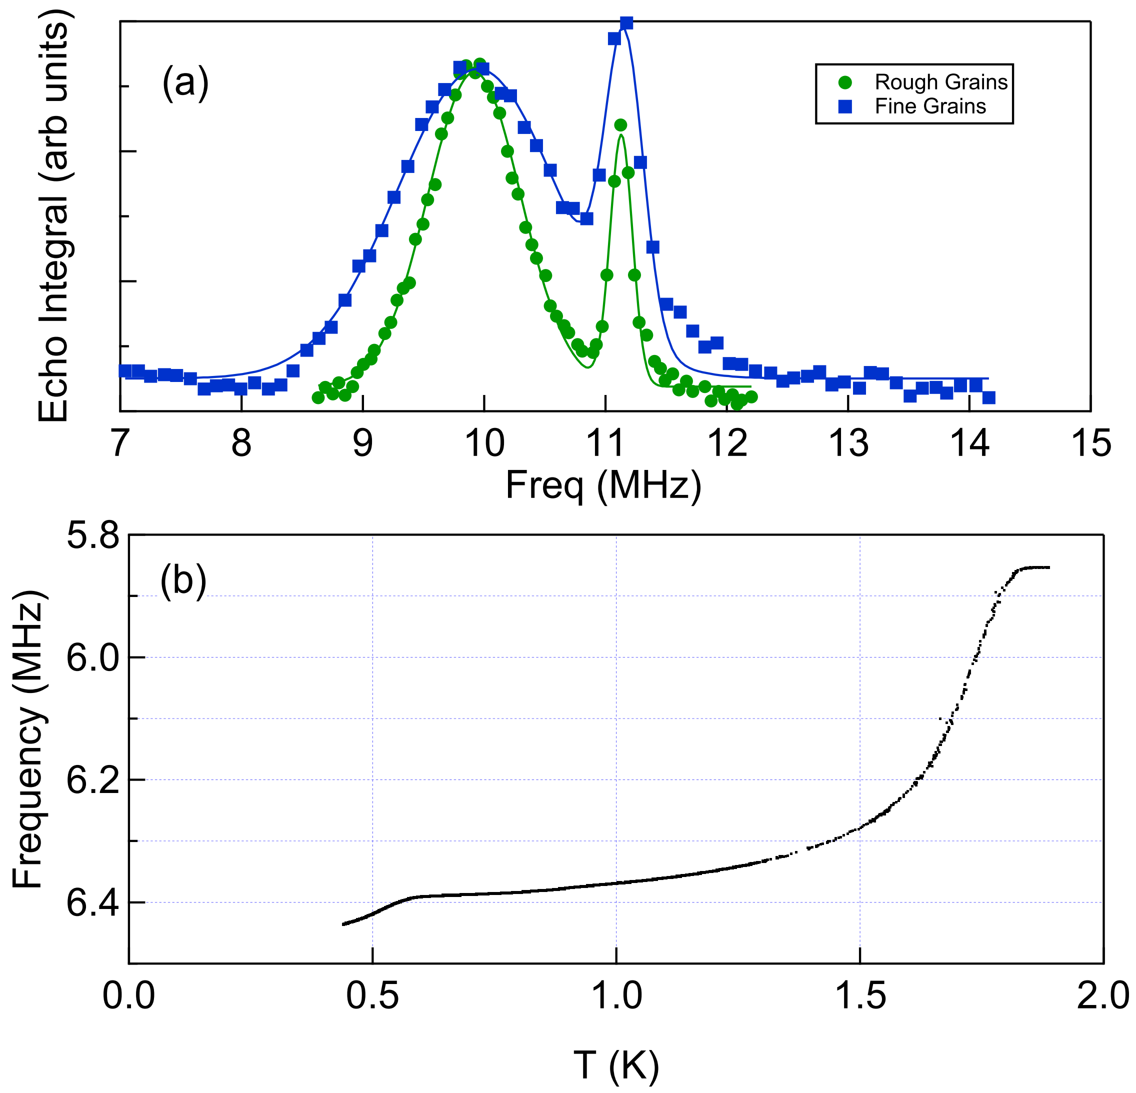


FIG. S1. (a) NQR spectrum of $^{69}$Ga(2) before and after grinding powder to 10$\mu$m size. Solid lines are fits. (b) AC susceptibility of $LaNiGa_2$ as a function of temperature, measured by the resonance frequency of a tuned circuit (note the axis direction is reversed).

## I. SAMPLE PREPARATION

Single crystals of $LaNiGa_2$ were grown via flux methods as described in [S1], and several crystals with sizes 100-300$\mu$m were ground and sieved to grain sizes $\sim 10$ $\mu$m to improve the signal to noise ratio in the superconducting state. The NQR spectrum of the $^{69}$Ga(2) site broadened by approximately 76% after grinding, as shown in Fig. S1 due to an increased distribution of electric field gradients due to strain. The AC magnetic susceptibility of the

powder was measured via detuning of the NQR resonant tank circuit, as shown in Fig. S1. $T_c \approx 1.83$ K was unaffected by the grinding process. There was a small response that appeared below 0.6 K whose origin remains unknown, but which may be associated with the presence of an impurity phase (possibly LaNiGa) [S2].

## II. NQR MEASUREMENTS

This material has a single La site, and the resonance frequencies are determined by the quadrupolar Hamiltonian:

$$\mathcal{H}_Q = \frac{h\nu_{zz}}{6}\left[3\hat{I}_z^2 - \hat{I}^2 + \eta(\hat{I}_x^2 - \hat{I}_y^2)\right] \tag{S1}$$

where $h$ is the Planck constant, $\hat{\mathbf{I}}$ is the nuclear spin angular momentum operator, $\eta = (\nu_{xx} - \nu_{yy})/\nu_{zz}$ is the asymmetry parameter, and $\nu_{\alpha\alpha} = 3eQV_{\alpha\alpha}/2I(2I-1)h$ are the principal values of the electric field gradient (EFG) tensor, $V_{\alpha\beta}$, (where $\alpha$ and $\beta$ stand for one of the three directions of the principal axes of the EFG tensor), $I = 7/2$ is the nuclear spin quantum number, and $Q$ is the nuclear quadrupolar moment. For the La site the principal direction lies along the crystalline $b$ axis with $\nu_{zz} = 1.65$ MHz and $\eta = 0.04$ [S2]. There are three transitions at frequencies $\sim n\nu_Q$, where $n = 1, 2, 3$ and $\nu_Q = \nu_{zz}\sqrt{1 + \eta^2/3}$ and the measurements were carried out at the $3\nu_Q \approx 5.060$ MHz transition. The spin-lattice relaxation rate, $T_1^{-1}$, was measured by the inversion recovery method. The recovery of the nuclear magnetization was fit to the standard expression for the $3\nu_Q$ transition for $I = 7/2$ with magnetic fluctuations: $M(t) = M_0\left(1 - 2f\sum_n A_n e^{-\alpha_n t/T_1}\right)$, where $M_0$ is the equilibrium nuclear magnetization, $f$ is the inversion fraction, $A_1 = 3/14$, $A_2 = 50/77$, $A_3 = 3/22$, $\alpha_1 = 3$, $\alpha_2 = 10$, $\alpha_3 = 21$.

## III. COHERENCE FACTORS

We begin by introducing the BdG Hamiltonian governing the electrons in terms of their free Dirac type dispersion as well as the pairing potential. This acts on an 8-dimensional space that we can think of as the tensor product of 3 copies of spin-$\frac{1}{2}$ Hilbert spaces corresponding to particle/hole, spin up/down, and band A/B with associated Pauli matrices $\lambda_i$,

$\sigma_i$, and $\tau_i$ respectively. Using this construction, we have

$$H_{BdG} = \sum_{\mathbf{k}} \Psi_{\mathbf{k}}^{\dagger} H(\mathbf{k}) \Psi_{\mathbf{k}}, \tag{S2}$$

$$H(\mathbf{k}) = \begin{bmatrix} h_0(\mathbf{k}) & \hat{\Delta} \\ \hat{\Delta}^{\dagger} & -h_0(\mathbf{k}) \end{bmatrix},$$

$$h_0(\mathbf{k}) = \mathbb{1}_2 \otimes \left( v_{\mathbf{k}} \cdot \mathbf{k} \mathbb{1}_2 + \gamma_{\mathbf{k}} \cdot \mathbf{k} \tau_x \right),$$

$$\Delta = (\mathbf{d} \cdot \sigma) i\sigma_y \otimes i\tau_y,$$

$$\Psi_k = \left( a_{\mathbf{k}\uparrow}, b_{\mathbf{k}\uparrow}, a_{\mathbf{k}\downarrow}, b_{\mathbf{k}\downarrow}, a_{-\mathbf{k}\uparrow}^{\dagger}, b_{-\mathbf{k}\uparrow}^{\dagger}, a_{-\mathbf{k}\downarrow}^{\dagger}, b_{-\mathbf{k}\downarrow}^{\dagger} \right).$$

Here we use parameters $v_{\mathbf{k}}$ and $\gamma_{\mathbf{k}}$ introduced in [S3]. Note, as mentioned in the main text, that dependence on $\mathbf{k}$ will be solely on its component perpendicular to the Fermi surface, so for brevity we supress the vectorial notation and refer to the perpendicular component by k. The vector $\mathbf{d} = \Delta \boldsymbol{\eta}$, where $\Delta$ is a scalar and $\boldsymbol{\eta}$ a unit vector, describes the mechanism through which electrons pair up by spin. We use the basis of electron creation and annihilation operators with momentum and spin labels associated with the A and B bands respectively. At this stage, we elect to consider vectors $\mathbf{d}$ that lie either in the $x-y$ plane or the $y-z$ plane in $\mathbb{C}^3$; i.e. $\mathbf{d} = (d_{x,r} + id_{x,i}, d_{y,r} + id_{y,i}, 0)$ or $\mathbf{d} = (0, d_{y,r} + id_{y,i}, d_{z,r} + id_{z,i})$. The $r$ and $i$ indices denote real and imaginary parts. With this choice, $H_{BdG}$ can be diagonal in the spin ($\sigma$) subspace with respect to either the $\sigma_z$ or the $\sigma_x$ eigenbasis. Additionally, note that with this choice, the pairing potential $\hat{\Delta}$ can be written as $(\Delta_r(\sigma) - i\Delta_i(\sigma)) \otimes \tau_y$, where:

$$\hat{\Delta}_r(\sigma) = c_j d_{j,i} \sigma_p - d_{y,r} \mathbb{1}_2; \; \hat{\Delta}_i(\sigma) = c_j d_{j,r} \sigma_p + d_{y,i} \mathbb{1}_2, \tag{S3}$$

and $j = x$ or $z$ with $c_j = \begin{cases} 1 & \text{if } j = x, \; p = z \\ -1 & \text{if } j = z, \; p = x \end{cases}$. Evidently, this pairing potential is diagonal. From here, we work in the $\lambda \otimes \tau$ subspace, which gives us an effective $4 \times 4$ model. We replace the operators $\Delta_r(\sigma)$ and $\Delta_i(\sigma)$ with their eigenvalues which we shall denote by $\delta_{jr,\pm} = \pm c_j d_{j,i} - d_{y,r}$ and $\delta_{ji,\pm} = \pm c_j d_{j,r} + d_{y,i}$, leading to:

$$H_{\text{eff}}(k) = v_k k \lambda \otimes \mathbb{1}_2 + \gamma_k k \lambda_z \otimes \tau_x + \delta_{jr,\pm} \lambda_x \otimes \tau_y + \delta_{ji,\pm} \lambda_y \otimes \tau_y. \tag{S4}$$

Here, one can check that $\lambda_z \otimes \tau_x$ commutes with $H_{\text{eff}}(k)$, so we now change basis from the standard basis to one consisting of eigenvectors of $\lambda_z \otimes \tau_x$, which are of the form $\frac{1}{\sqrt{2}} \begin{pmatrix} 1 \\ 0 \end{pmatrix} \otimes$

$\begin{pmatrix} 1 \\ \pm 1 \end{pmatrix}$ and $\frac{1}{\sqrt{2}}\begin{pmatrix} 0 \\ 1 \end{pmatrix} \otimes \begin{pmatrix} 1 \\ \pm 1 \end{pmatrix}$. In changing basis, we obtain the following Hamiltonian, which we shall denote by $\tilde{H}(k)$, where the Pauli matrices also carry a tilde to emphasize the basis change.

$$\tilde{H}(k) = -\gamma_k k \tilde{\lambda}_z \otimes \mathbb{1}_2 + v_k k \mathbb{1}_2 \otimes \tilde{\tau}_z + \tilde{\lambda}_z \otimes (\delta_{jr,\pm}\tilde{\tau}_y - \delta_{ji,\pm}\tilde{\tau}_x) \tag{S5}$$

$$= \mp\gamma_k k \mathbb{1}_2 + v_k k \tilde{\tau}_z \pm \delta_{jr,\pm}\tilde{\tau}_y \mp \delta_{ji,\pm}\tilde{\tau}_x \tag{S6}$$

Equation (S6) reveals that our transformed Hamiltonian is now diagonal in the $\tilde{\lambda}$ subspace, which means that we can reduce to an effective $2 \times 2$ model in $\tilde{\tau}$ space. We now rewrite (S6) in a manner that suggests how to diagonalize the $2 \times 2$ system.

$$\tilde{H}(k) \pm \gamma_k k \mathbb{1}_2 = W_\pm \left( w_{\pm\pm} \cdot \tilde{\tau} \right) \tag{S7}$$

In the line above, we introduce the constant $W_\pm = \sqrt{(v_k k)^2 + \Delta^2(1 \pm |\mathbf{q}|)}$. The $\pm$ here distinguishes between spin up($+$) and spin down($-$), and $\mathbf{q} = i\boldsymbol{\eta} \times \boldsymbol{\eta}^*$. This precise dependence of $\Delta^2(1 \pm |\mathbf{q}|)$ can be obtained by explicitly calculating the normalization factor $W_\pm$ from equation (S7). The unit vector $w_{\pm\pm}$ takes the form $w_{\pm\pm} = \frac{1}{W_\pm}(\mp\delta_{ji,\pm}, \pm\delta_{jr,\pm}, v_k k)$. We now define spherical coordinates $\theta_\pm = \arccos\left(\frac{v_k k}{W_\pm}\right)$ and $\varphi_{\pm\pm} = \operatorname{sgn}(\pm\delta_{jr,\pm}) \arccos\left(\frac{\mp\delta_{ji,\pm}}{\Delta}\right)$. In terms of these angular parameters, the eigenvectors of (8) with energies $E_{\mp\pm\pm}(k) = \mp\gamma_k k \pm W_\pm$ are as written below.

$$|t_{\pm\pm-}\rangle = \begin{pmatrix} -e^{-i\varphi_{\pm\pm}} \sin\left(\frac{\theta_\pm}{2}\right) \\ \cos\left(\frac{\theta_\pm}{2}\right) \end{pmatrix} \tag{S8}$$

$$|t_{\pm\pm+}\rangle = \begin{pmatrix} \cos\left(\frac{\theta_\pm}{2}\right) \\ e^{i\varphi_{\pm\pm}} \sin\left(\frac{\theta_\pm}{2}\right) \end{pmatrix}. \tag{S9}$$

To generate the eigenvectors of the initial $8 \times 8$ model, we first let $|+\rangle = \begin{pmatrix} 1 \\ 0 \end{pmatrix}$ and $|-\rangle = \begin{pmatrix} 0 \\ 1 \end{pmatrix}$, and the color will denote these as eigenvectors of the $\tilde{\lambda}$ subspace (black) or the $\sigma$ subspace (cyan).

$$|T_{\pm\pm\pm}\rangle_j = |\pm\rangle \otimes |\pm\rangle_j \otimes |t_{\pm\pm\pm}\rangle \tag{S10}$$

We use the notation here that the subscript $j$ denotes $|\pm\rangle_j$ to be the eigenvectors of $\sigma_j$ with $j = x$ or $z$. We will now use these eigenvectors $|T_{\pm\pm\pm}\rangle_j$ to express the Bogoliubov quasiparticle creation and annihilation operators in terms of $a$ and $b$ electron creation and annihilation operators, and we will drop the $j$ subscript for brevity of notation. Letting $u_{k\pm} = -e^{-i\varphi_{+\pm}} \sin\left(\frac{\theta_\pm}{2}\right)$ and $v_{k\pm} = \cos\left(\frac{\theta_\pm}{2}\right)$ be the so-called coherence factors (note the switched convention compared to standard BCS Theory), we are able to derive the following expressions:

$$\alpha_{\mathbf{k}\pm} = v_{\mathbf{k}\pm}(a_{\mathbf{k}\pm} - b_{\mathbf{k}\pm}) - u^*_{\mathbf{k}\pm}(a^\dagger_{-\mathbf{k}\pm} + b^\dagger_{-\mathbf{k}\pm}) \tag{S11}$$

$$\beta^\dagger_{-\mathbf{k}\pm} = u_{\mathbf{k}\pm}(a_{\mathbf{k}\pm} - b\mathbf{k}\pm) + v_{\mathbf{k}\pm}(a^\dagger_{-\mathbf{k}\pm} + b^\dagger_{-\mathbf{k}\pm}) \tag{S12}$$

One can check that these operators satisfy the fermionic anticommutation relations. Note that the general form of these quasiparticle operators is close to the standard BCS form, barring the presence of two bands A and B. However, the basis change we implemented causes $a$ and $b$ electrons to mix, a consequence of the $\gamma_k k$ term in the Hamiltonian. The electron operators may now be expressed in terms of the Bogoliubov operators:

$$a_{\mathbf{k}\pm} = u^*_{\mathbf{k}\pm}\beta^\dagger_{-\mathbf{k}\pm} + v_{\mathbf{k}\pm}\alpha_{\mathbf{k}\pm} - u^*_{-\mathbf{k}\pm}\alpha^\dagger_{-\mathbf{k}\pm} + v_{-\mathbf{k}\pm}\beta_{\mathbf{k}\pm} \tag{S13}$$

$$b_{\mathbf{k}\pm} = -u^*_{-\mathbf{k}\pm}\alpha^\dagger_{-\mathbf{k}\pm} + v_{-\mathbf{k}\pm}\beta_{\mathbf{k}\pm} - u^*_{\mathbf{k}\pm}\beta^\dagger_{-\mathbf{k}\pm} - v_{\mathbf{k}\pm}\alpha_{\mathbf{k}\pm} \tag{S14}$$

With these operator expressions, we now move on to computing the nuclear relaxation rate, $T_1^{-1}$, with reference to the $S^+$ term of the Hyperfine Hamiltonian. In this calculation, the nuclear wavefunction is approximated as constant, so calculating $T_1^{-1}$ effectively involves using Fermi's Golden Rule to calculate scattering amplitudes associated with electron states. Towards this end, we introduce the operator,

$$S^+_{\mathbf{k},\mathbf{k'}}(\phi) = (\cos(\phi)a^\dagger_{\mathbf{k}\downarrow} + \sin(\phi)b^\dagger_{\mathbf{k}\downarrow})(\cos(\phi)a_{\mathbf{k'}\uparrow} + \sin(\phi)b_{\mathbf{k'}\uparrow}). \tag{S15}$$

This operator describes electron scattering from momentum **k'** to **k** where spin is flipped, and the parameter $\phi$ is introduced to allow us to vary the relative weight of $a$ versus $b$ electrons in the scattering process. This angle is given by $\tan\phi = 2A_aA_b/(A_a^2 + A_b^2)$, where $A_{a,b}$ are the hyperfine couplings to the two bands. As mentioned before, we invoke Fermi's Golden Rule and $T_1^{-1}$ involves calculating $\sum_{i,f} \left|\langle f|S^+_{\mathbf{k},\mathbf{k'}}(\phi)|i\rangle\right|^2$, where $i$ and $f$ are the initial and final states of the scattering process which both correspond to states with only one

Bogoliubov quasiparticle present. Thus, we sum over initial states featuring an $\alpha_{\mathbf{k'}\pm}$ or a $\beta_{\mathbf{k'}\pm}$ excitation and final states featuring an $\alpha_{\mathbf{k}\pm}$ or a $\beta_{\mathbf{k}\pm}$ excitation. Before proceeding however, we now need to acknowledge the role played by the choice of $j = x$ or $z$. In the case that $j = z$, we may directly write (S15) in terms of (S13) and (S14). This lets us calculate the scattering amplitudes directly, and this is presented in the next section. Remark again that we will express the dependence of these expressions on $\mathbf{k}$ as dependence on its component perpendicular to the Fermi surface, denoted as just k.

### A. j = z

By direct computation, express the electron creation and annihilation operators in (S15), and then read off the scattering amplitudes to obtain,

$$
\begin{aligned}
A_{\alpha\uparrow\to\alpha\downarrow}(k,k') &= v_{k\downarrow}v_{k'\uparrow}\left(1-\sin(2\phi)\right) \\
A_{\alpha\downarrow\to\alpha\uparrow}(k,k') &= u^*_{k\uparrow}u_{k'\downarrow}\left(1+\sin(2\phi)\right) \\
A_{\beta\uparrow\to\beta\downarrow}(k,k') &= v_{-k\downarrow}v_{-k'\uparrow}\left(1+\sin(2\phi)\right) \\
A_{\beta\downarrow\to\beta\uparrow}(k,k') &= u^*_{-k\uparrow}u_{-k'\downarrow}\left(1-\sin(2\phi)\right) \\
A_{\alpha\uparrow\to\beta\downarrow}(k,k') &= v_{-k\downarrow}v_{k'\uparrow}\cos(2\phi) \\
A_{\alpha\downarrow\to\beta\uparrow}(k,k') &= u^*_{-k\uparrow}u_{k'\downarrow}\cos(2\phi) \\
A_{\beta\uparrow\to\alpha\downarrow}(k,k') &= v_{k\downarrow}v_{-k'\uparrow}\cos(2\phi) \\
A_{\beta\downarrow\to\alpha\uparrow}(k,k') &= u^*_{k\uparrow}u_{-k'\downarrow}\cos(2\phi)
\end{aligned} \tag{S16}
$$

The next section outlines the differences imposed by the condition $j = x$.

### B. j=x

The reason that the calculation of these scattering elements becomes trickier now is that they involve transitions from up spin to down spin particles while our Bogoliubov quasiparticles are labeled by $S_x$ eigenvalues. We make use of the relation:

$$c_{k,\uparrow} = \frac{1}{\sqrt{2}}\left(c_{k,+} + c_{k,-}\right) \tag{S17}$$

$$c_{k,\downarrow} = \frac{1}{\sqrt{2}}\left(c_{k,+} - c_{k,-}\right), \tag{S18}$$

where the $c_k$ operator here can be either $a_k$ or $b_k$. With this transformation, we can write $S^{+}_{k,k'}(\phi)$, but first note the forms of the operators $S^{-}_{k,k'}$ and $S^{z}_{k,k'}$:

$$
\begin{aligned}
S^{-}_{k,k'}(\phi) &= (\cos(\phi)a^{\dagger}_{k\uparrow} + \sin(\phi)b^{\dagger}_{k\uparrow})(\cos(\phi)a_{k'\downarrow} + \sin(\phi)b_{k'\downarrow}), \\
S^{z}_{k,k'}(\phi) &= \frac{1}{2}\sum_{s} s(\cos(\phi)a^{\dagger}_{ks} + \sin(\phi)b^{\dagger}_{ks})(\cos(\phi)a_{k's} + \sin(\phi)b_{k's}),
\end{aligned} \tag{S19}
$$

where $s = \pm 1$ denotes up/down spin. In this case where our natural spin basis is that of $\sigma_x$, we can express $S^{+}_{k,k'}(\phi)$ in the following way.

$$
\begin{aligned}
S^{+,\uparrow\backslash\downarrow}_{k,k'}(\phi) &= S^{z,\pm}_{k,k'}(\phi) + \frac{1}{2}\left(S^{-,\pm}_{k,k'}(\phi) - S^{+,\pm}_{k,k'}(\phi)\right) \\
&= S^{z,\pm}_{k,k'}(\phi) - iS^{y,\pm}_{k,k'}(\phi)
\end{aligned} \tag{S20}
$$

The notation for the $S$ operators in the equation above is as follows. Those operators with $\uparrow \backslash \downarrow$ as a superscript involve spin matrices written in the usual $z$-basis. Those with $\pm$ in the superscript involve the exact same matrices, elementwise, except the "$z$-basis" here actually corresponds to the $x$-basis. Consequently, the scattering amplitudes associated with $S^{+,\uparrow\backslash\downarrow}_{k,k'}(\phi)$ can be calculated by considering scattering between $\alpha_{\pm}$ particles and $\beta_{\pm}$ particles. Furthermore, we can use the same scattering amplitudes found in the previous section, except the $\uparrow\rightarrow\downarrow$ scattering and vice versa will refer to $+ \rightarrow -$ scattering and vice versa. With this in mind, we have the following amplitudes that will contribute to our calculation of $T_1^{-1}$.

$$
\begin{aligned}
A_{\alpha\pm\rightarrow\alpha\pm}(k,k') &= \frac{1}{2}\left(v_{k\pm}v_{k'\pm}(1-\sin(2\phi)) - u^{*}_{k\pm}u_{k'\pm}(1+\sin(2\phi))\right) \\
A_{\beta\pm\rightarrow\beta\pm}(k,k') &= \frac{1}{2}\left(v_{-k\pm}v_{-k'\pm}(1+\sin(2\phi)) - u^{*}_{-k\pm}u_{-k'\pm}(1-\sin(2\phi))\right) \\
A_{\alpha\pm\rightarrow\beta\pm}(k,k') &= \frac{1}{2}\cos(2\phi)\left(u^{*}_{-k\pm}u_{k'\pm} - v_{-k\pm}v_{k'\pm}\right) \\
A_{\beta\pm\rightarrow\alpha\pm}(k,k') &= \frac{1}{2}\cos(2\phi)\left(u^{*}_{k\pm}u_{-k'\pm} - v_{k\pm}v_{-k'\pm}\right) \\
A_{\alpha+\rightarrow\alpha-}(k,k') &= \frac{1}{2}\left(u^{*}_{k-}u_{k'+}(1+\sin(2\phi)) - v_{k-}v_{k'+}(1-\sin(2\phi))\right) \\
A_{\alpha-\rightarrow\alpha+}(k,k') &= \frac{1}{2}\left(v_{k+}v_{k'-}(1-\sin(2\phi)) - u^{*}_{k+}u_{k'-}(1+\sin(2\phi))\right)
\end{aligned} \tag{S21}
$$

$$A_{\beta+\to\beta-}(k,k') = \frac{1}{2}\left(u^*_{-k-}u_{-k'+}(1-\sin(2\phi)) - v_{-k-}v_{-k'+}(1+\sin(2\phi))\right)$$
$$A_{\beta-\to\beta+}(k,k') = \frac{1}{2}\left(v_{-k+}v_{-k'-}(1+\sin(2\phi)) - u^*_{-k+}u_{-k'-}(1-\sin(2\phi))\right)$$
$$A_{\alpha+\to\beta-}(k,k') = \frac{1}{2}\cos(2\phi)\left(u^*_{-k-}u_{k'+} - v_{-k-}v_{-k'+}\right)$$
$$A_{\alpha-\to\beta+}(k,k') = \frac{1}{2}\cos(2\phi)\left(v_{-k+}v_{k'-} - u^*_{-k+}u_{k'-}\right)$$
$$A_{\beta+\to\alpha-}(k,k') = \frac{1}{2}\cos(2\phi)\left(u^*_{k-}u_{-k'+} - v_{k-}v_{-k'+}\right)$$
$$A_{\beta-\to\alpha+}(k,k') = \frac{1}{2}\cos(2\phi)\left(v_{k+}v_{-k'-} - u^*_{k+}u_{-k'-}\right)$$

These amplitudes can be decomposed into two subsets of scattering processes: those which preserve the $x$ component of spin and those which flip this. The first four equations involve the processes that preserve spin, and these are in fact the same amplitudes that appear in the calculation of ultrasonic attenuation for either orientation of $\mathbf{d}$ that we have considered. The existence of spin-preserving, i.e. gap preserving, scattering is what distinguishes the behavior of quasiparticle scattering when $\mathbf{d}$ has a component along the $z$-axis.

### C. Relaxation Rate

With these amplitudes in hand, we may now proceed to calculate the nuclear relaxation rate using Fermi's Golden Rule. Following the notes of Arovas and Wu, we sum over $k$, $k'$, and spins $s, s' = \pm 1$ of the following (where $s, s'$ can correspond to either the $z$ or $x$ bases):

$$\sum_{\mathbf{k},\mathbf{k'},s,s'} |A_{\alpha s'\to\alpha s}(\mathbf{k},\mathbf{k'})|^2 f_{\alpha,\mathbf{k},s}(1-f_{\alpha,\mathbf{k'},s'})\delta(E_{\alpha,\mathbf{k'},s'} - E_{\alpha,\mathbf{k},s} - \hbar\omega) + \quad \text{(S22)}$$
$$|A_{\beta s'\to\beta s}(\mathbf{k},\mathbf{k'})|^2 f_{\beta,\mathbf{k},s}(1-f_{\beta,\mathbf{k'},s'})\delta(E_{\beta,\mathbf{k'},s'} - E_{\beta,\mathbf{k},s} - \hbar\omega)$$

where $f_{\alpha,\mathbf{k},s}$ and $f_{\beta,\mathbf{k},s}$ denote the Fermi-Dirac functions corresponding to alpha and beta particles respectively with momentum $\mathbf{k}$ and spin $s$. This labeling convention is also used to index the energies in the argument of the delta function. Note that the strongest enhancement of relaxation rate will occur due to processes that do not require quasiparticles to hop across the two gaps, i.e. the spin component is preserved. These are more energetically favorable and are only possible if $\mathbf{d}$ is perpendicular to the $\mathbf{x}$ direction (see the first four equations of Eq. S21). To introduce temperature dependence into the formation of a superconducting gap, we let $\Delta(T) = \Delta_0(T)\sqrt{1-\left(\frac{\gamma_k}{v_k}\right)^2}\sqrt{1\pm|\sin\theta_\eta|}$, where $\Delta_0(T)$ has

the temperature dependence given by the solution to the self-consistency equation for the singlet BCS Theory gap,

$$\int_0^\infty d\epsilon\,\left[\frac{\tanh\left(\sqrt{\epsilon^2+\Delta^2}/2T\right)}{\sqrt{\epsilon^2+\Delta^2}}-\frac{1}{\sqrt{\epsilon^2+\Delta(0)^2}}\right], \tag{S23}$$

where $\Delta(0)$ is the $T=0$ value of the parameter such that $T_c=1$. $\Delta_0(T)$ is then obtained by scaling the solution to the equation above such that $\Delta_0(0)$ takes on any given value.

## IV. VARIATION WITH NUCLEAR FREQUENCY

Figure S2 shows the calculated $T_1^{-1}$ for several different values of the nuclear resonance frequency within the INT model for $\mathbf{d}\perp\mathbf{x}$. Smaller frequencies enhance the coherence peak, but the experimental measurement frequency is $\omega_N=10^{-4}$. Note that in the INT model, with two distinct gaps it is still possible to have enhancement of $T_1^{-1}$ below $T_c$ due to scattering processes that preserve the spin component, so reducing the nuclear frequency enables this enhancement to increase to a point where it can fit the experimental data more closely. However, such a fit requires an unphysical nuclear frequency of $\hbar\omega_N/k_BT_c=10^{-12}$ to achieve good agreement with the data (the experimental value is $10^{-4}$). This suggests a very sensitive peak with notable time reversal symmetry breaking, as discussed in the main text.

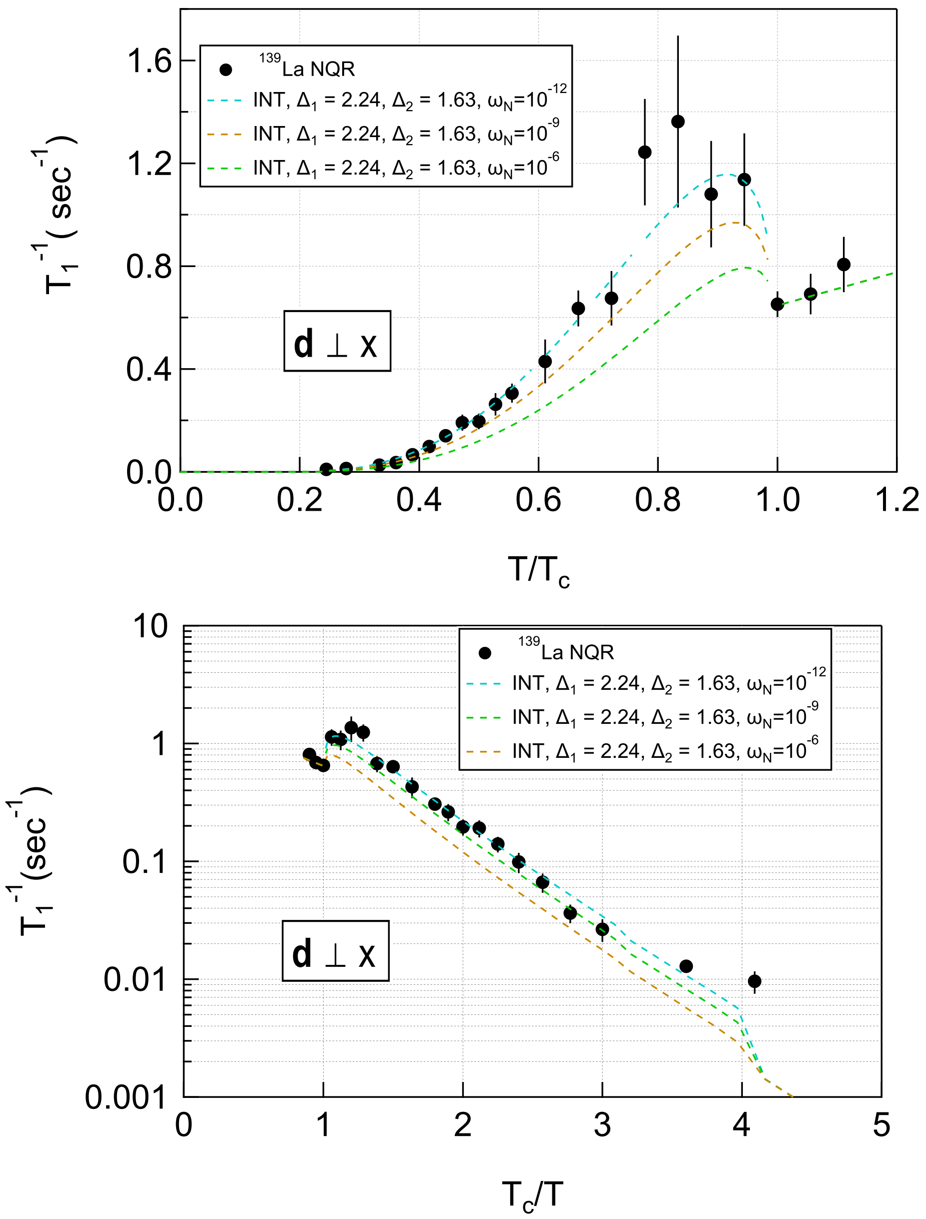


FIG. S2. Calculated $T_1^{-1}$ versus temperature and inverse temperature within the INT model for various values of the measurement frequency, $\omega_N$. The solid points are the experimental measurements.

## V. d-VECTOR OF FORM $(a, i, 0)$

As described in the main text, one class of pairing vector $\mathbf{d}$ we consider is of the form $\mathbf{d}_a = \frac{\Delta_0}{\sqrt{1+a^2}}(a, i, 0)$. With the parameter $\phi$ from the scattering operator $S(\phi)$ set to $0.05\pi$ and nuclear frequency set to $\omega_N = 10^{-4}$, we find best fit parameters $\Delta_0 = 1.9$, $a = 5 \times 10^{-5}$,

indicated by the hexagon in Fig. S3(a). The fitting was performed by calculating the reduced $\chi^2$, comparing theoretical calculations with experimental data. Note that we restrict the temperature range, in units of $T/T_c$, to $T > 0.4$ to emphasize the fitting of the peak of $(T_1)^{-1}$. Furthermore, these best fit parameters yield two superconducting gaps of 1.8599 and 1.8601, which are nearly identical. As one deviates from $\Delta_0 = 1.9$, $a = 5 \times 10^{-5}$, the fit quality worsens, and Fig. S3(b) illustrates examples of this. If one were to consider plots of $(T_1)^{-1}$ generated by parameters outside the blue envelope in the heat map of Fig. S3(a), the fit to the peak would deteriorate noticeably in comparison to even the curve with $\chi^2 = 2.4$.

Importantly, the heat map illustrates that for larger $\Delta_0$, which scales the two gaps of the model, better fits arise from using smaller $a$, causing the splitting of the two gaps to be reduced. As one decreases $\Delta_0$, increasing $a$ beyond 0 has a smaller effect on the difference in the two gaps, i.e. time reversal symmetry breaking. Thus, the $a$ values that fit the experiment up to $\chi^2 < 4$ get larger as $\Delta_0$ decreases. However, as $\Delta_0$ reaches below 1.7, not only does the fit of the INT model worsen, but the range of "better fitting" $a$ values becomes narrower as well. Ultimately, aside from these details, the range of $a$ studied here induces minimal TRSB, which is the important takeaway from solving the INT model.

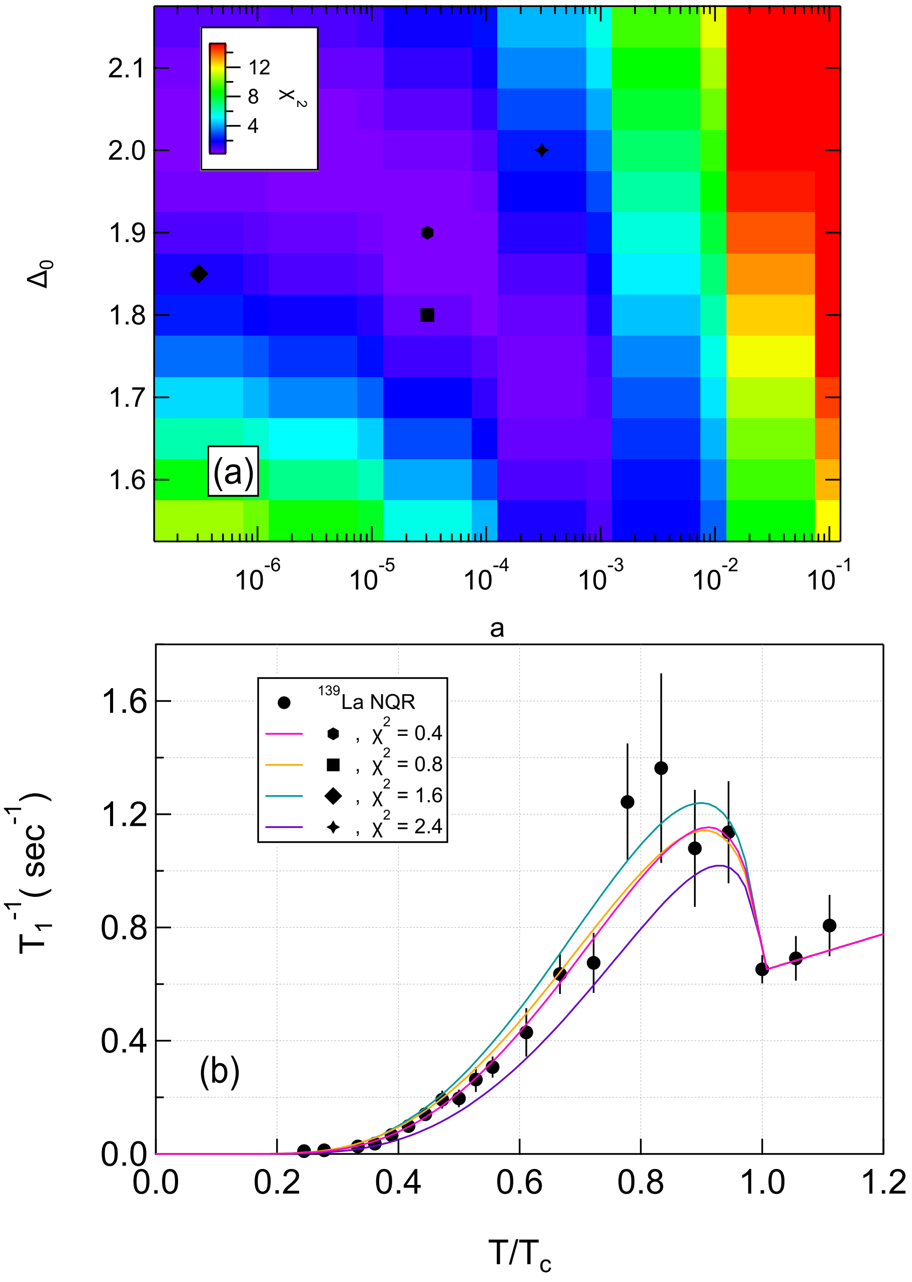


FIG. S3. Panel (a) shows $\chi^2$ as a function of fitting parameters $a$ and $\Delta_0$ as heat map. The four points correspond to different curves in panel (b). The best fit is given by solid hexagon (magenta curve). In both panels, the nuclear frequency in units of $k_B T_c$ is $10^{-4}$.

[S1] J. R. Badger, Y. Quan, M. C. Staab, S. Sumita, A. Rossi, K. P. Devlin, K. Neubauer, D. S. Shulman, J. C. Fettinger, P. Klavins, S. M. Kauzlarich, D. Aoki, I. M. Vishik, W. E. Pickett, and V. Taufour, Dirac lines and loop at the fermi level in the time-reversal symmetry breaking superconductor $LaNiGa_2$, Communications Physics **5**, 22 (2022).

[S2] P. Sherpa, I. Vinograd, Y. Shi, S. A. Sreedhar, C. Chaffey, T. Kissikov, M.-C. Jung, A. S. Botana, A. P. Dioguardi, R. Yamamoto, M. Hirata, G. Conti, S. Nemsak, J. R. Badger, P. Klavins, I. Vishik, V. Taufour, and N. J. Curro, Absence of strong magnetic fluctuations or interactions in the normal state of $LaNiGa_2$, Phys. Rev. B **109**, 125113 (2024).

[S3] Y. Quan, V. Taufour, and W. E. Pickett, Nonsymmorphic band sticking in a topological superconductor, Phys. Rev. B **105**, 064517 (2022).
